# Supplementary material for: CryoBench: Diverse and challenging datasets for the heterogeneity problem in cryo-EM
Source: arXiv:2408.05526 source file (2025-01-16)
Supplement: Supplementary file 1 [file 21_pose_error.tex]

\usepackage{subcaption} % Add this line to your preamble

\begin{figure}[h]
    \centering
    \begin{minipage}{0.3\textwidth}
        \centering
        \includegraphics[width=\textwidth,trim={0 0 0 2.5cm},clip]{SI/SI_Figures/pngs/pose_error/confhet1_pose_residuals_median_align_right_flip2.pdf}
        \subcaption{IgG-1D}\label{fig:pose_error_distribution_a}
    \end{minipage}\hfill
    \begin{minipage}{0.3\textwidth}
        \centering
        \includegraphics[width=\textwidth,trim={0 0 0 2.5cm},clip]{SI/SI_Figures/pngs/pose_error/confhet2_pose_residuals_median_align_right_flip2.pdf}
        \subcaption{IgG-RL}\label{fig:pose_error_distribution_b}
    \end{minipage}
    \newline
    \begin{minipage}{0.3\textwidth}
        \centering
        \includegraphics[width=\textwidth,trim={0 0 0 2.5cm},clip]{SI/SI_Figures/pngs/pose_error/mixhet_pose_residuals_median_align_right_flip2.pdf}
        \subcaption{Tomotwin-100}\label{fig:pose_error_distribution_c}
    \end{minipage}\hfill
    \begin{minipage}{0.3\textwidth}
        \centering
        \includegraphics[width=\textwidth,trim={0 0 0 2.5cm},clip]{SI/SI_Figures/pngs/pose_error/md_pose_residuals_median_align_right_flip2.pdf}
        \subcaption{Spike-MD}\label{fig:pose_error_distribution_d}
    \end{minipage}
    \caption{{\bf Pose error distributions.}}
    \label{fig:pose_error_distribution}
\end{figure}
