# Supplementary material for: CryoBench: Diverse and challenging datasets for the heterogeneity problem in cryo-EM
Source: arXiv:2408.05526 source file (2025-01-16)
Supplement: Supplementary file 2 [file 001_conf_het_1_snr001.tex]

\begin{table*}[t]
  \centering
  \footnotesize
  \resizebox{1\textwidth}{!}{
      \begin{tabular}{c|c|c|c|c|c|c|c|c}
        \toprule
        
        \multirow{2}{*}{\textbf{Method}} & \multicolumn{4}{|c|}{\textbf{SNR 0.005}} & \multicolumn{4}{c}{\textbf{SNR 0.001}} \\
        \cmidrule(r){2-9}
        & \multicolumn{2}{|c|}{No Mask} & \multicolumn{2}{c}{Mask} & \multicolumn{2}{|c|}{No Mask} & \multicolumn{2}{c}{Mask} \\
        % \cmidrule(r){2-9}
        & Mean (std) & Median & Mean (std) & Median & Mean (std) & Median & Mean (std) & Median \\
        \midrule
        CryoDRGN & 0.345 (0.003) & 0.345 & 0.355 (0.003) & 0.355 & 0.296 (0.002) & 0.296 & 0.316 (0.003) & 0.316 \\
        DrgnAI-fixed & 0.346 (0.008) & 0.351 & 0.36 (0.001) & 0.36 & 0.293 (0.008) & 0.288 & 0.317 (0.002) & 0.317 \\
        Opus-DSD & 0.254 (0.006) & 0.254 & 0.255 (0.006) & 0.255 & 0.251 (0.006) & 0.252 & 0.252 (0.006) & 0.253 \\
        3DFlex & 0.226 (0.003) & 0.226 & 0.226 (0.003) & 0.226 & 0.224 (0.006) & 0.225 & 0.224 (0.006) & 0.225  \\
        3DVA & 0.269 (0.024) & 0.253 & 0.307 (0.027) & 0.289 & 0.209 (0.017) & 0.202 & 0.256 (0.019) & 0.249 \\
        RECOVAR & 0.384 (0.001) & 0.384 & 0.385 (0.001) & 0.385 & 0.358 (0.002) & 0.358 & 0.361 (0.002) & 0.361 \\
        3D Class & 0.269 (0.024) & 0.253 & 0.307 (0.027) & 0.289 & 0.209 (0.017) & 0.202 & 0.256 (0.019) & 0.249 \\
        \midrule

        CryoDRGN2 & 0.285 (0.085) & 0.326 & 0.289 (0.086) & 0.33 & 0.141 (0.022) & 0.149 & 0.161 (0.03) & 0.173 \\
        DrgnAI-abinit & 0.289 (0.097) & 0.341 & 0.295 (0.099) & 0.348 & 0.159 (0.01) & 0.159 & 0.177 (0.011) & 0.177 \\
        3D Class (\textit{ab initio}) & 0.13 (0.044) & 0.164 & 0.138 (0.048) & 0.174 & 0.094 (0.036) & 0.086 & 0.105 (0.044) & 0.091 \\
        \bottomrule
      \end{tabular}
    }
    \caption{\textbf{Higher and Highest noise of Conf-het-1.} }
    \label{tab:supp1_noise}
\end{table*}
