# Supplementary material for: CryoBench: Diverse and challenging datasets for the heterogeneity problem in cryo-EM
Source: arXiv:2408.05526 source file (2025-01-16)
Supplement: Supplementary file 3 [file 004_table_conf-het-1_embd.tex]

\begin{table*}[t]
  \centering
  \footnotesize
  \resizebox{1\textwidth}{!}{
      \begin{tabular}{c|c|c|c|c|c|c|c|c}
        \toprule
        
        \multirow{3}{*}{\textbf{Method}} & \multicolumn{4}{|c|}{\textbf{Embeddings Conf-het-1}} & \multicolumn{4}{c}{\textbf{Embeddings Conf-het-2}} \\
        \cmidrule(r){2-9}
        & \multicolumn{2}{|c|}{$\mathrm{pMN}$ [\%]} & \multicolumn{2}{c|}{Information Imbalance}  & \multicolumn{2}{|c|}{$\mathrm{pMN}$ [\%]} & \multicolumn{2}{c}{Information Imbalance} \\
        % \cmidrule(r){2-5} \cmidrule(l){7-10}
        & k=1\% & k=5\% & $\Delta(gt\rightarrow e)$ & $\Delta(e\rightarrow gt)$ &  k=1\% & k=5\% & $\Delta(gt\rightarrow e)$ & $\Delta(e\rightarrow gt)$  \\
        \midrule
        CryoDRGN & 12.00(0.03)& 39.08 (0.07)& & &19.03 (0.15)	& 17.08 (0.08) & & \\
        
        DrgnAI-fixed & 28.87 (0.08) & 74.53 (0.11)& & &53.25 (0.33)	& 27.55 (0.05) & & \\
        
        Opus-DSD & 26.75 (0.05)& 70.56 (0.11)& & &\textbf{ 71.35 (0.17)}	& \textbf{31.37 (0.06)} & & \\
        
        3DFlex & 24.97 (0.06) & 61.75 (0.12)& & &22.81 (0.21)	& 21.62 (0.09)  & & \\
        
        3DVA & 11.97 (0.03) & 44.96 (0.04) & & & 7.30 (0.06)	& 15.25 (0.07) & & \\
        
        RECOVAR & \textbf{30.42 (0.08)}& \textbf{78.81 (0.07)}& & & 18.39 (0.09)	& 23.16 (0.10) & & \\
        \midrule

        CryoDRGN2 & 12.40 (0.05)& 45.83 (0.16)& & & 5.02 (0.04)	& 11.15 (0.08) & & \\
        DrgnAI-abinit & \textbf{19.30 (0.06)}& \textbf{57.27 (0.17) }& & & \textbf{25.71 ( 0.10)}	& \textbf{21.82 (0.08)} & & \\
        \bottomrule
      \end{tabular}
    }
    \caption{\textbf{Quantitative embedding metrics for conf-het-1 and conf-het-2.} \textit{Percentage of matching neighbors} ($\mathrm{pMN}$) for two neighborhoods k=$1$,$5$\%. The mean from five independent subsets is presented, and standard deviation of the mean is shown in parenthesis.  \textit{Information imbalance}  }
    \label{tab:tab1_joint}
\end{table*}
