# Supplementary material for: CryoBench: Diverse and challenging datasets for the heterogeneity problem in cryo-EM
Source: arXiv:2408.05526 source file (2025-01-16)
Supplement: Supplementary file 4 [file clustering_ari.tex]

\begin{table}[t]
  \centering
  \resizebox{0.5\textwidth}{!}{
      \begin{tabular}{c|c|c|c|c}
        \toprule
         \multirow{2}{*}{\textbf{Method}} & \multicolumn{2}{c|}{\textbf{Ribosembly}} & \multicolumn{2}{c}{\textbf{Tomotwin-100}} \\
        \cmidrule(r){2-5}
        & ARI & AMI & ARI & AMI \\
        \midrule
        CryoDRGN & 0.873 & \underline{0.935} & \textbf{0.956} & \textbf{0.983} \\
        DRGN-AI-fixed & 0.624 & 0.771 & \underline{0.791} & \underline{0.906} \\
        Opus-DSD & \underline{0.891} & 0.934 & 0.500 & 0.781 \\
        3DVA & 0.666 & 0.823 & 0.058 & 0.335 \\
        RECOVAR & \textbf{0.968} & \textbf{0.976} & 0.315 & 0.649 \\
        
        \midrule

        CryoDRGN2 & 0.529 & 0.618 & \textbf{0.116} & \textbf{0.374} \\
        DRGN-AI & \textbf{0.644} & \textbf{0.729} & 0.086 & 0.275 \\ 
        \bottomrule
      \end{tabular}
    }
    \vspace{5pt}
    \captionof{table}{\textbf{K-Means Clustering Accuracy.} Adjusted Rand Index (ARI) and Adjusted Mutual Information (AMI) between true structural labels and predicted labels for each particle. Predicted labels are obtained by running $k$-means clustering on the particle latents, with $k$ set to the number of ground truth structures. These findings align with those previously reported for neighborhood similarity, as shown in Table 2.  }
    \label{tab:supp_ari}
\end{table}
