# Supplementary material for: CryoBench: Diverse and challenging datasets for the heterogeneity problem in cryo-EM
Source: arXiv:2408.05526 source file (2025-01-16)
Supplement: Supplementary file 5 [file 11_information_imbalance_old.tex]

\begin{figure*}[t]
    \centering % trim = left bottom right top
    
    \begin{subfigure}{0.16\textwidth}
        \includegraphics[width=\textwidth,trim={1.5cm 0 4.2cm 1.2cm}, clip]{SI/SI_Figures/pngs/information_imbalance/confhet1_information_imbalance_pose.pdf}
        \includegraphics[width=\textwidth,trim={1.5cm 0 2.9cm 1.25cm}, clip]{SI/SI_Figures/pngs/information_imbalance/confhet1_information_imbalance_pose_zoom.pdf}
        \caption{IgG-1D}
        \label{fig:pose_sub1}
    \end{subfigure}
    \hfill
    \begin{subfigure}{0.16\textwidth}
        \includegraphics[width=\textwidth,trim={1.5cm 0 4.2cm 1.2cm}, clip]{SI/SI_Figures/pngs/information_imbalance/confhet2_information_imbalance_pose.pdf}
        \includegraphics[width=\textwidth,trim={1.4cm 0 2.9cm 1.25cm}, clip]{SI/SI_Figures/pngs/information_imbalance/confhet2_information_imbalance_pose_zoom.pdf}
        \caption{IgG-RL}
        \label{fig:pose_sub2}
    \end{subfigure}
    \hfill
    \begin{subfigure}{0.16\textwidth}
        \includegraphics[width=\textwidth,trim={2.0cm 0 4.2cm 1.2cm}, clip]{SI/SI_Figures/pngs/information_imbalance/assemble_information_imbalance_pose.pdf}
        \includegraphics[width=\textwidth,trim={2.0cm 0 2.9cm 1.25cm}, clip]{SI/SI_Figures/pngs/information_imbalance/assemble_information_imbalance_pose_zoom.pdf}
        \caption{Ribosembly}
        \label{fig:pose_sub3}
    \end{subfigure}
    \hfill
    \begin{subfigure}{0.16\textwidth}
        \includegraphics[width=\textwidth,trim={1.3cm 0 4.2cm 1.2cm}, clip]{SI/SI_Figures/pngs/information_imbalance/mix_information_imbalance_pose.pdf}
        \includegraphics[width=\textwidth,trim={1.15cm 0 2.7cm 1.25cm}, clip]{SI/SI_Figures/pngs/information_imbalance/mix_information_imbalance_pose_zoom.pdf}
        \caption{T.twin-100}
        \label{fig:pose_sub4}
    \end{subfigure}
    \hfill
    \begin{subfigure}{0.16\textwidth}
        \includegraphics[width=\textwidth,trim={0.8cm 0 4.2cm 1.2cm}, clip]{SI/SI_Figures/pngs/information_imbalance/md_information_imbalance_pose.pdf}
        \includegraphics[width=\textwidth,trim={0.675cm 0 2.0cm 1.25cm}, clip]{SI/SI_Figures/pngs/information_imbalance/md_information_imbalance_pose_zoom.pdf}
        \caption{Spike-MD}
        \label{fig:pose_sub5}
    \end{subfigure}
    \hfill
    \begin{subfigure}{0.16\textwidth}
        \includegraphics[width=\textwidth,trim={0.1cm -1.75cm 0 0 }, clip]{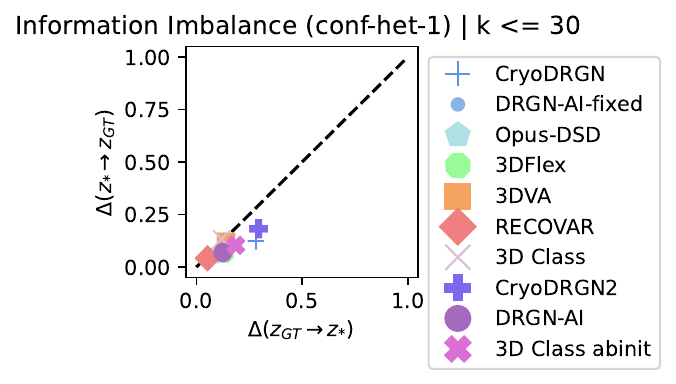}
        % \caption{} % omit for no label
        \label{fig:si_information_imbalance_ctf_legend}
    \end{subfigure}
    
    \caption{\textbf{Pose Information Imbalance}. In full view ($[0,1]^2$; top row) and zoomed in (bottom row).}
    \label{fig:si_information_imbalance_pose}
\end{figure*}

\begin{figure*}[t]
    \centering % trim = left bottom right top
    
    \begin{subfigure}{0.16\textwidth}
        \includegraphics[width=\textwidth,trim={1.5cm 0 4.2cm 1.2cm}, clip]{SI/SI_Figures/pngs/information_imbalance/confhet1_information_imbalance_ctf.pdf}
        \includegraphics[width=\textwidth,trim={1.5cm 0 2.9cm 1.25cm}, clip]{SI/SI_Figures/pngs/information_imbalance/confhet1_information_imbalance_ctf_zoom.pdf}
        \caption{IgG-1D}
        \label{fig:ctf_sub1}
    \end{subfigure}
    \hfill
    \begin{subfigure}{0.16\textwidth}
        \includegraphics[width=\textwidth,trim={1.5cm 0 4.2cm 1.2cm}, clip]{SI/SI_Figures/pngs/information_imbalance/confhet2_information_imbalance_ctf.pdf}
        \includegraphics[width=\textwidth,trim={1.4cm 0 2.9cm 1.25cm}, clip]{SI/SI_Figures/pngs/information_imbalance/confhet2_information_imbalance_ctf_zoom.pdf}
        \caption{IgG-RL}
        \label{fig:ctf_sub2}
    \end{subfigure}
    \hfill
    \begin{subfigure}{0.16\textwidth}
        \includegraphics[width=\textwidth,trim={2.0cm 0 4.2cm 1.2cm}, clip]{SI/SI_Figures/pngs/information_imbalance/assemble_information_imbalance_ctf.pdf}
        \includegraphics[width=\textwidth,trim={2.0cm 0 2.9cm 1.25cm}, clip]{SI/SI_Figures/pngs/information_imbalance/assemble_information_imbalance_ctf_zoom.pdf}
        \caption{Ribosembly}
        \label{fig:ctf_sub3}
    \end{subfigure}
    \hfill
    \begin{subfigure}{0.16\textwidth}
        \includegraphics[width=\textwidth,trim={1.3cm 0 4.2cm 1.2cm}, clip]{SI/SI_Figures/pngs/information_imbalance/mix_information_imbalance_ctf.pdf}
        \includegraphics[width=\textwidth,trim={1.15cm 0 2.7cm 1.25cm}, clip]{SI/SI_Figures/pngs/information_imbalance/mix_information_imbalance_ctf_zoom.pdf}
        \caption{T.twin-100}
        \label{fig:ctf_sub4}
    \end{subfigure}
    \hfill
    \begin{subfigure}{0.16\textwidth}
        \includegraphics[width=\textwidth,trim={0.8cm 0 4.2cm 1.2cm}, clip]{SI/SI_Figures/pngs/information_imbalance/md_information_imbalance_ctf.pdf}
        \includegraphics[width=\textwidth,trim={0.675cm 0 2.0cm 1.25cm}, clip]{SI/SI_Figures/pngs/information_imbalance/md_information_imbalance_ctf_zoom.pdf}
        \caption{Spike-MD}
        \label{fig:ctf_sub5}
    \end{subfigure}
    \hfill
    \begin{subfigure}{0.16\textwidth}
        \includegraphics[width=\textwidth,trim={0.1cm -1.75cm 0 0 }, clip]{SI/SI_Figures/pngs/information_imbalance/information_imbalance_legend.pdf}
        % \caption{} % omit for no label
        \label{fig:si_information_imbalance_ctf_legend}
    \end{subfigure}
    
    \caption{\textbf{CTF Information Imbalance}. In full view ($[0,1]^2$; top row) and zoomed in (bottom row).}
    \label{fig:si_information_imbalance_ctf}
\end{figure*}

\begin{figure*}[t]
    \centering % trim = left bottom right top
    \includegraphics[width=0.45\textwidth,trim={0 0 0cm 0cm}, clip]{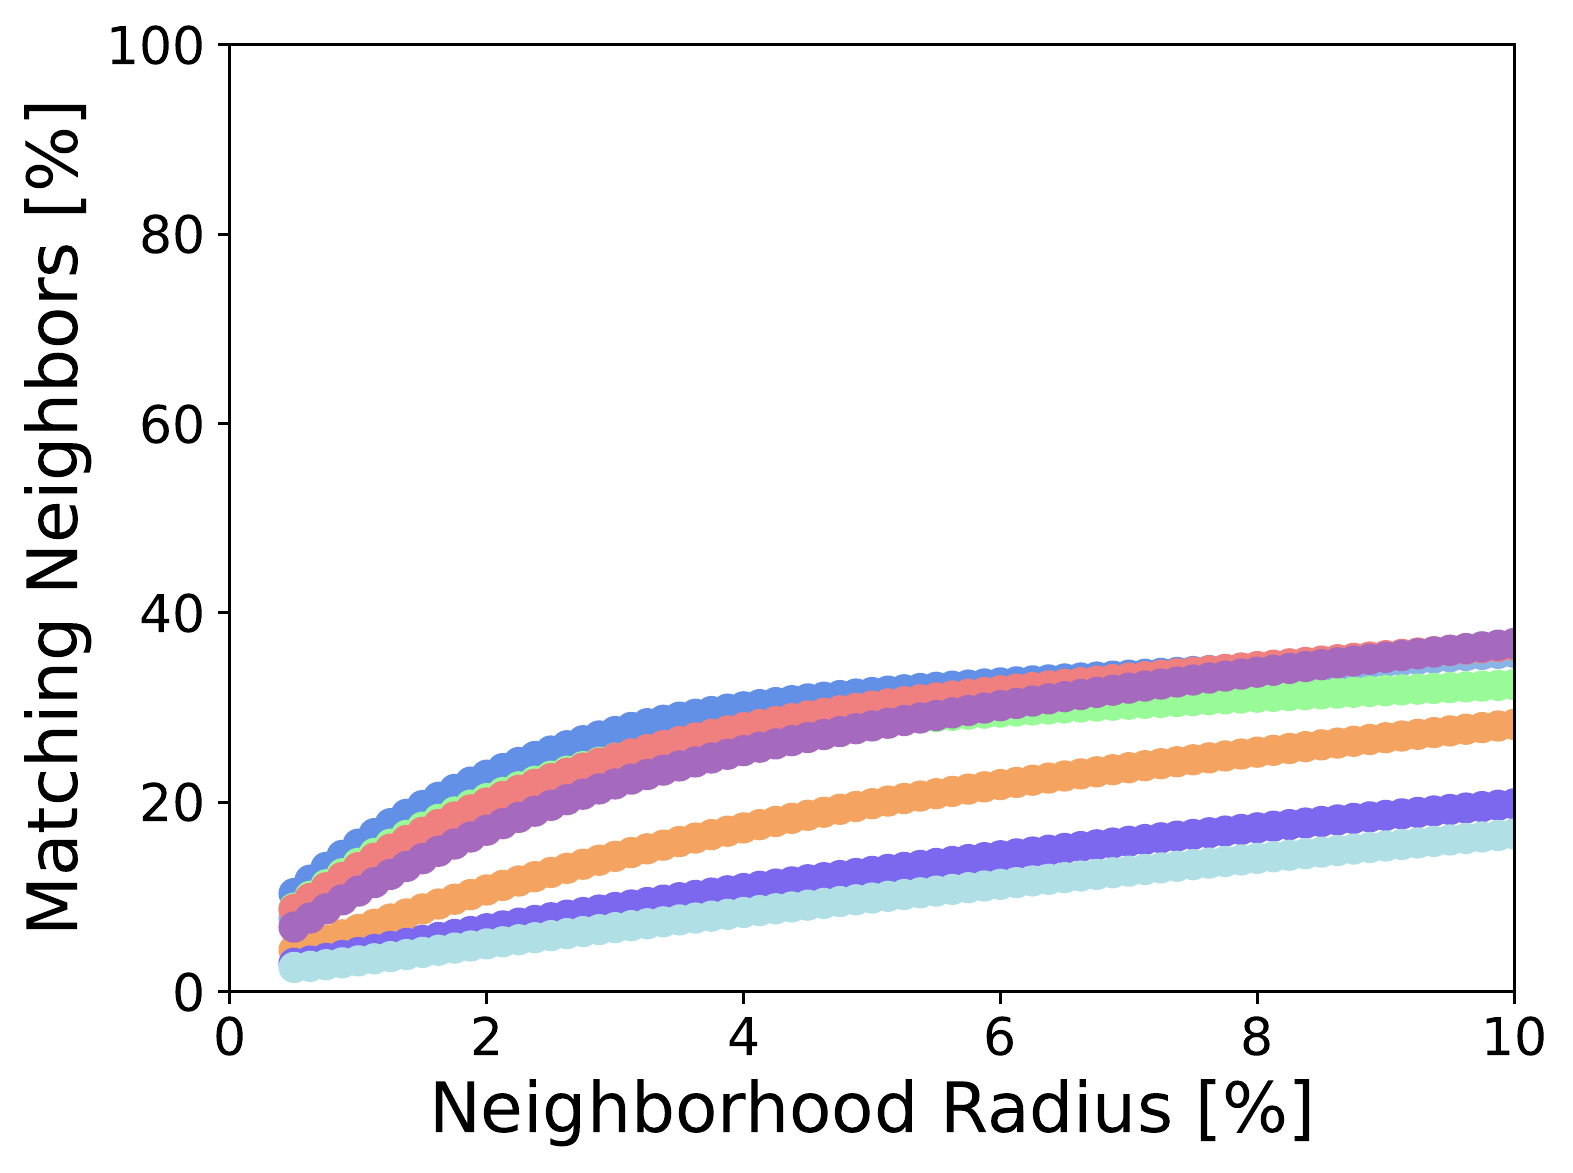}
    \includegraphics[width=0.45\textwidth,trim={0 0 0cm 0.75cm}, clip]{SI/SI_Figures/pngs/information_imbalance/md_information_imbalance.pdf}
   % \includegraphics[width=0.2\textwidth,trim={0 0 0 0}, clip]{SI/SI_Figures/pngs/information_imbalance/md_information_imbalance_legend.pdf}

    \caption{\textbf{Embedding metric results for the Spike-MD dataset} (left) Neighborhood similarity as a function of the neighborhood radius [\%]. (right) Information Imbalance. CryoDRGN2 (not visible) is underneath Opus-DSD.}
    \label{fig:si_MD_embd_metrics}
\end{figure*}
